# Supplementary material for: Semantic Tracklets: An Object-Centric Representation for Visual Multi-Agent Reinforcement Learning
Source: arXiv:2108.03319 source file (2021-08-06)
Supplement: Supplementary file 1 [file sec_supp.tex]

\clearpage

\appendix

\setcounter{table}{0}
\setcounter{figure}{0}

{\noindent\Large\textbf{Appendix}}

\vspace{0.3cm}
\noindent We discuss the following in the appendix:
\begin{enumerate}
\item In~\hyperref[sec:supp_island]{\secref{sec:supp_gfootabll}}, we provide results of semantic tracklets and the baseline on additional visual GFootball tasks. 
\item In~\hyperref[sec:supp_island]{\secref{sec:supp_island}}, we provide results of semantic tracklets and the baseline on an additional environment, \ie, a visual version of classic Stag Hunt game~\cite{Peysakhovich19}.
\item In~\hyperref[sec:supp_impl]{\secref{sec:supp_impl}}, we provide implementation details of the system, \ie, the detection and tracking pipeline, as well as the RL model and training details. 
\item In~\hyperref[sec:supp_plot]{\secref{sec:supp_plot}}, we provide training curves of controlling one, three, five, and ten agents on GFootball {\em 11 \vs 11} game and training curves on VMPE tasks for both semantic tracklets and baselines.
\end{enumerate} 

\noindent In additional files we also provide:
\vspace{-0.1cm}
 \begin{itemize}
 \itemsep0.1em
 \item Videos of the learned policies (see directory `\texttt{videos}')
 \item Python implementation of our approach (see directory `\texttt{code}')
 \end{itemize}

\input{supp_gfootball}
\input{supp_island}
\input{supp_implement}
\input{supp_plot}
